# Supplementary material for: Exploring Diffusion Time-steps for Unsupervised Representation Learning
Source: arXiv:2401.11430 source file (2024-01-21)
Supplement: Supplementary file 1 [file fig_ffhq-supp.tex]

\begin{figure}[!tbp]
  \centering
  \includegraphics[width=1.0\linewidth]{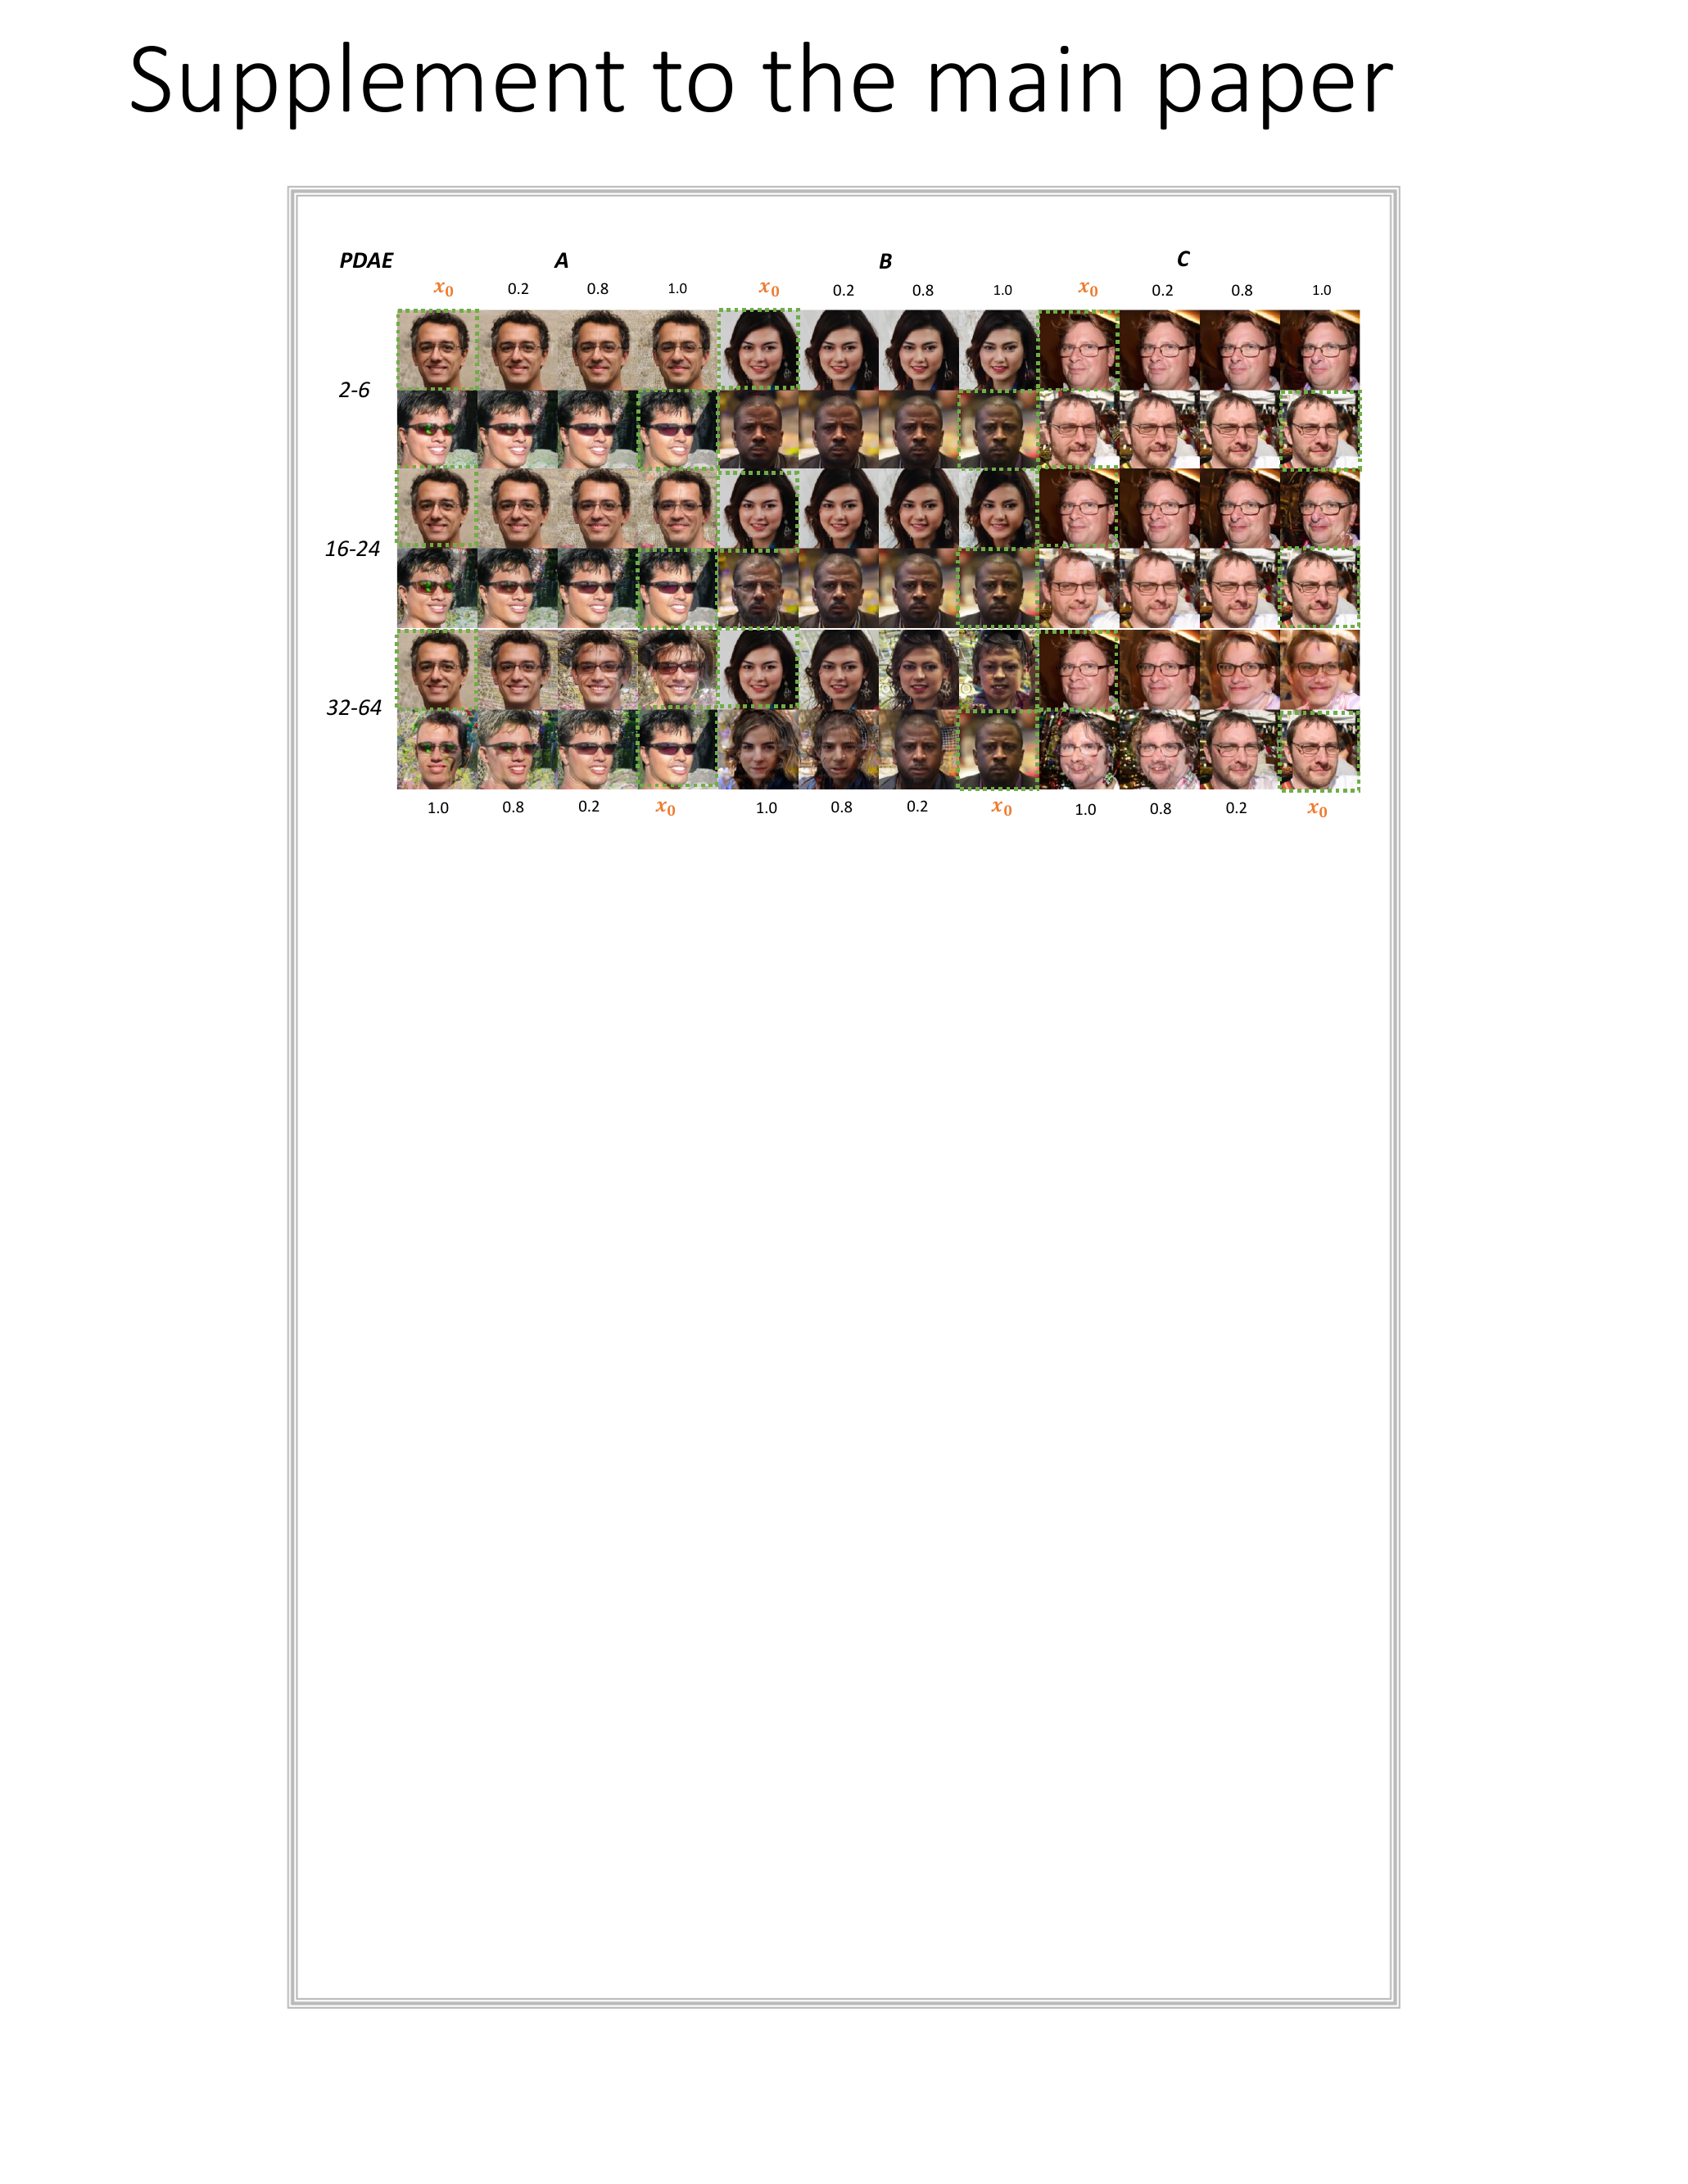}
  \caption{Counterfactual generations results with PDAE on FFHQ. Supplementary to Figure 5 in the main paper. }
  \label{suppfig:ffhq-supp}
  \vspace{-4mm}
\end{figure}
