# Supplementary material for: Exploring Diffusion Time-steps for Unsupervised Representation Learning
Source: arXiv:2401.11430 source file (2024-01-21)
Supplement: Supplementary file 2 [file figure7_supp.pdf]

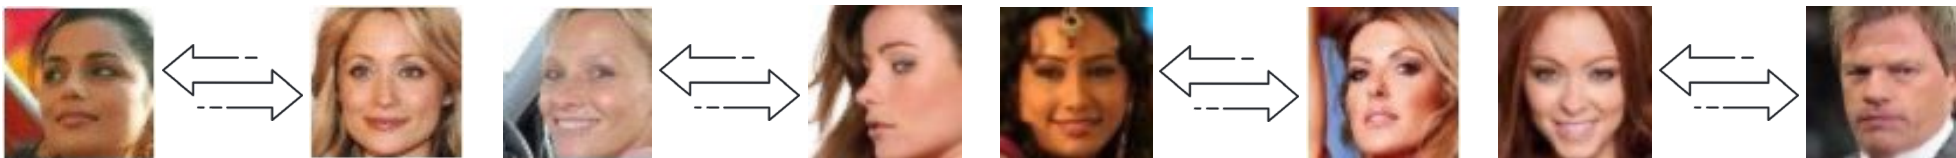

$\beta$ -TCVAE

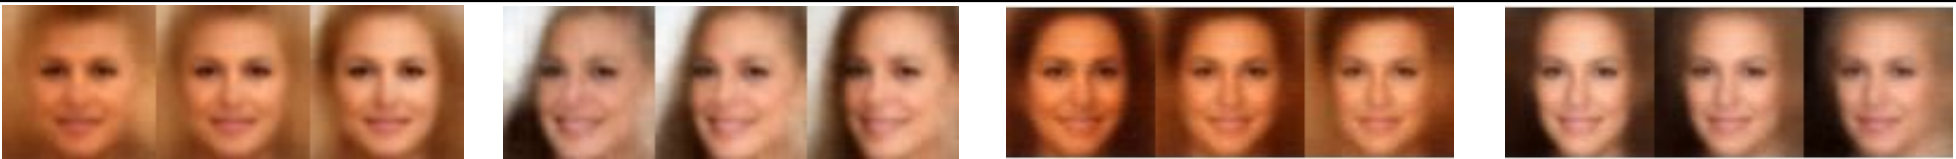

IB-GAN

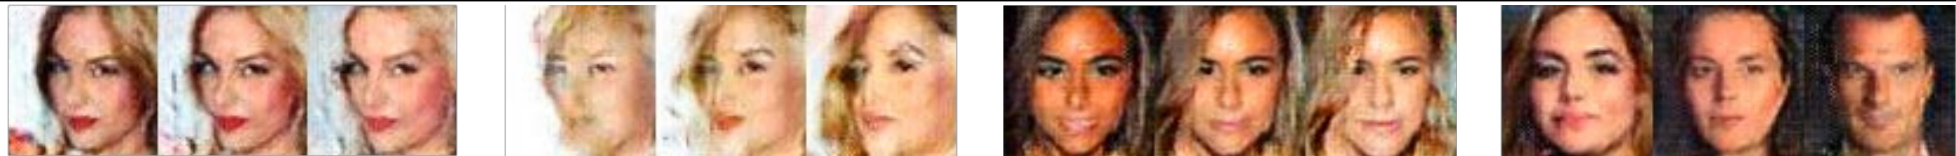

Diff-AE

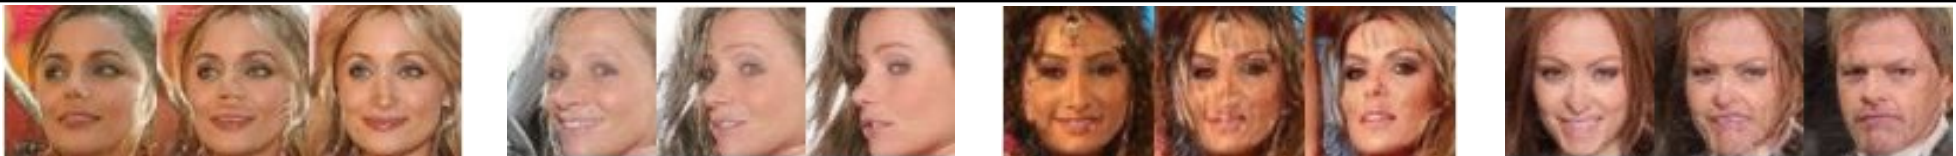

PDAE

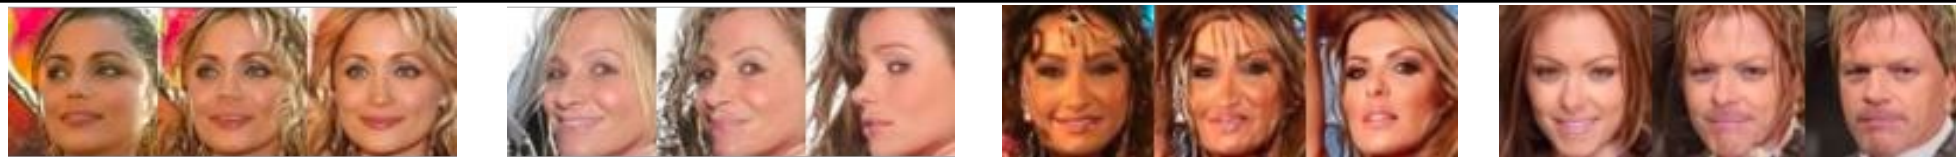

DiTi

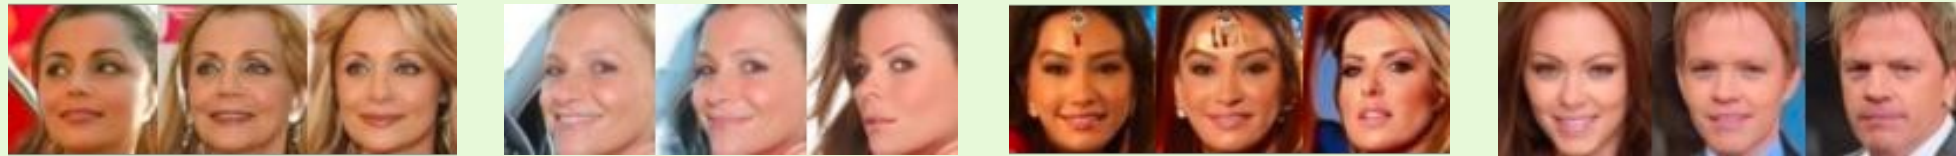

Template

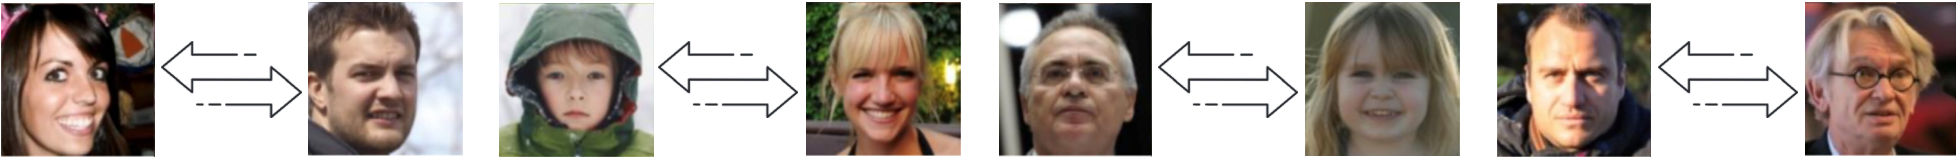

|         |  |  |  |  |  |  |
|---------|--|--|--|--|--|--|
| Diff-AE |  |  |  |  |  |  |
| PDAE    |  |  |  |  |  |  |
| DiTi    |  |  |  |  |  |  |

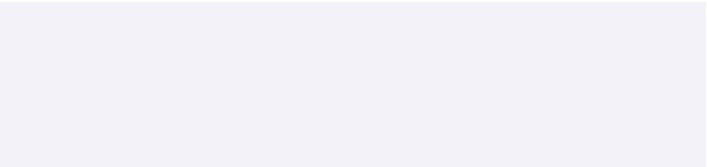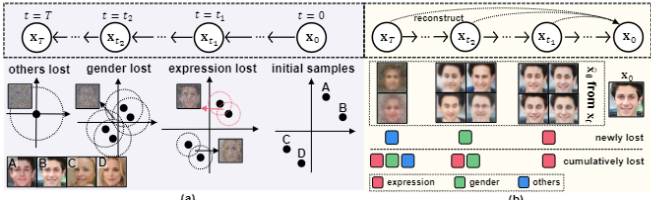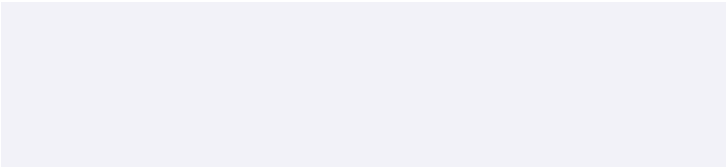

# CelebA full-dim interp

ori pairs:

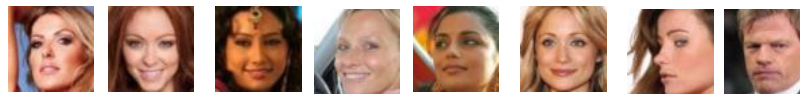

exp03\_baseline\_unequalseg\_test\_3477\_19421

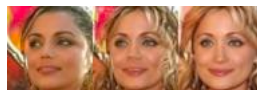

exp03\_pdae64stop\_unequalseg\_test\_3477\_19421

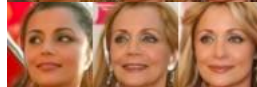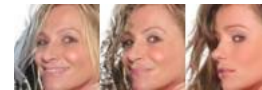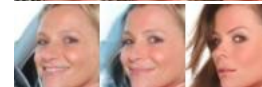

test\_4167\_1846

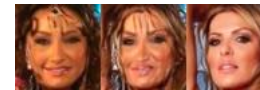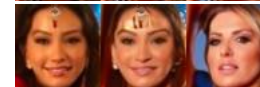

test\_5513\_8591

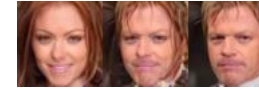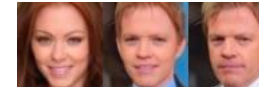

test\_8127\_17143
